# Supplementary material for: Arbitrary Volumetric Refocusing of Dense and Sparse Light Fields
Source: arXiv:2502.19238 source file (2025-02-26)
Supplement: Supplementary file 1 [file 7_appendix.tex]

\begin{figure*}[]
    \centering
    
    \begin{subfigure}[c]{0.29\textwidth}
         \centering
         \caption*{Middle SAI}
        %  \label{fig:y equals x}
     \end{subfigure}
     \hspace{0.1cm}
    \begin{subfigure}[c]{0.29\textwidth}
         \centering
         \caption*{Dense LF multi arbitrary-volume refocused image}
        %  \label{fig:y equals x}
     \end{subfigure}
     \hspace{0.1cm}
     \begin{subfigure}[c]{0.29\textwidth}
         \centering
         \caption*{Sparse LF multi arbitrary-volume refocused image}
        %  \label{fig:three sin x}
     \end{subfigure}

    \begin{subfigure}[t]{0.29\textwidth}
         \centering
         \includegraphics[width=\textwidth]{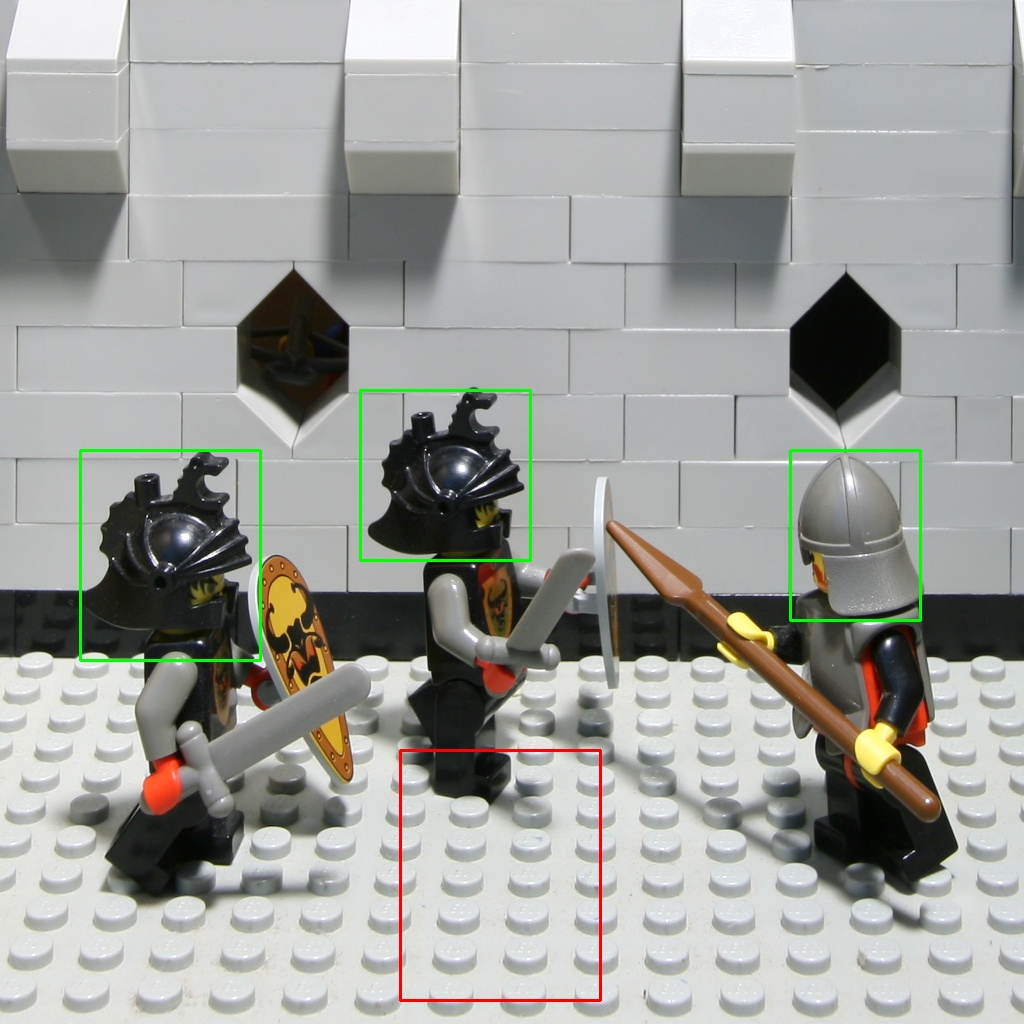}
        %  \caption{\small Evetar Lens M13B0618W}
        %  \label{fig:y equals x}
     \end{subfigure}
     \hspace{0.1cm}
    \begin{subfigure}[t]{0.29\textwidth}
         \centering
         \includegraphics[width=\textwidth]{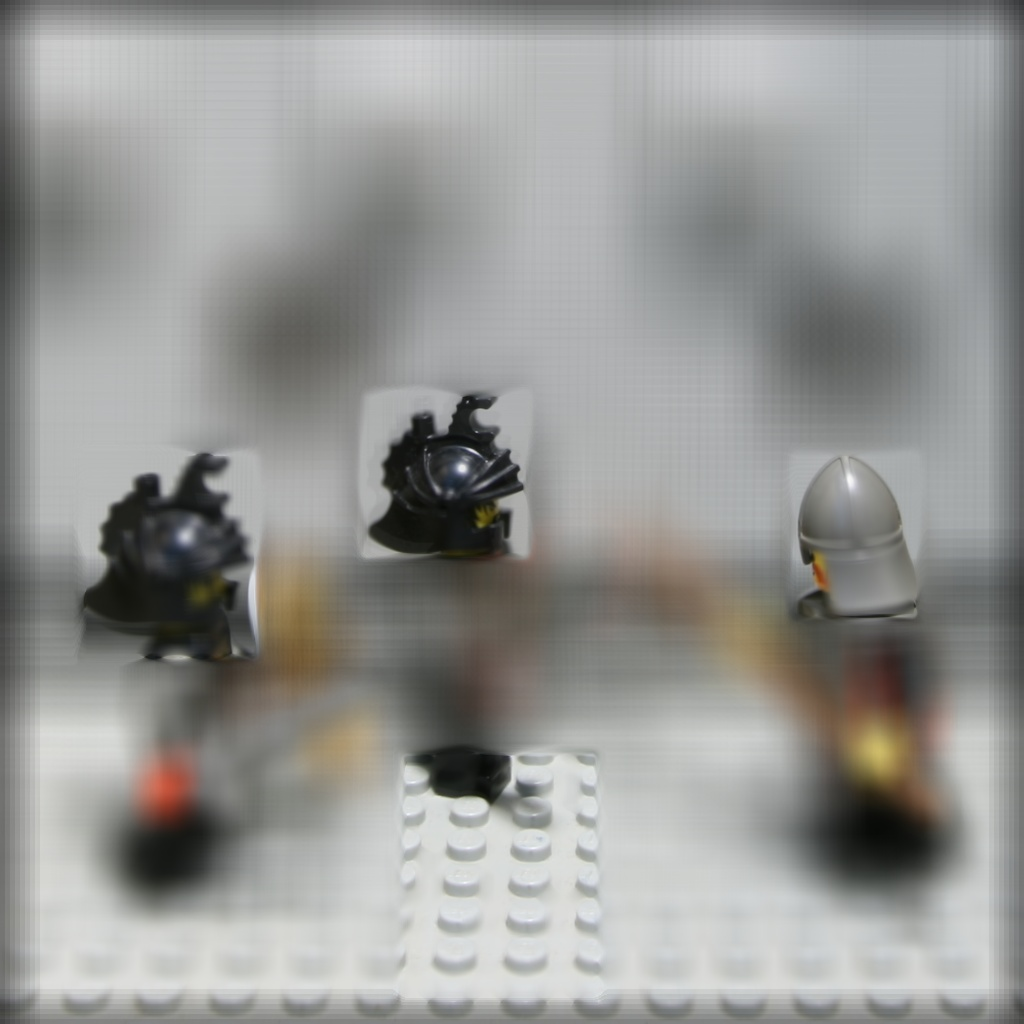}
         \caption{}
        %  \label{fig:y equals x}
     \end{subfigure}
     \hspace{0.1cm}
     \begin{subfigure}[t]{0.29\textwidth}
         \centering
         \includegraphics[width=\textwidth]{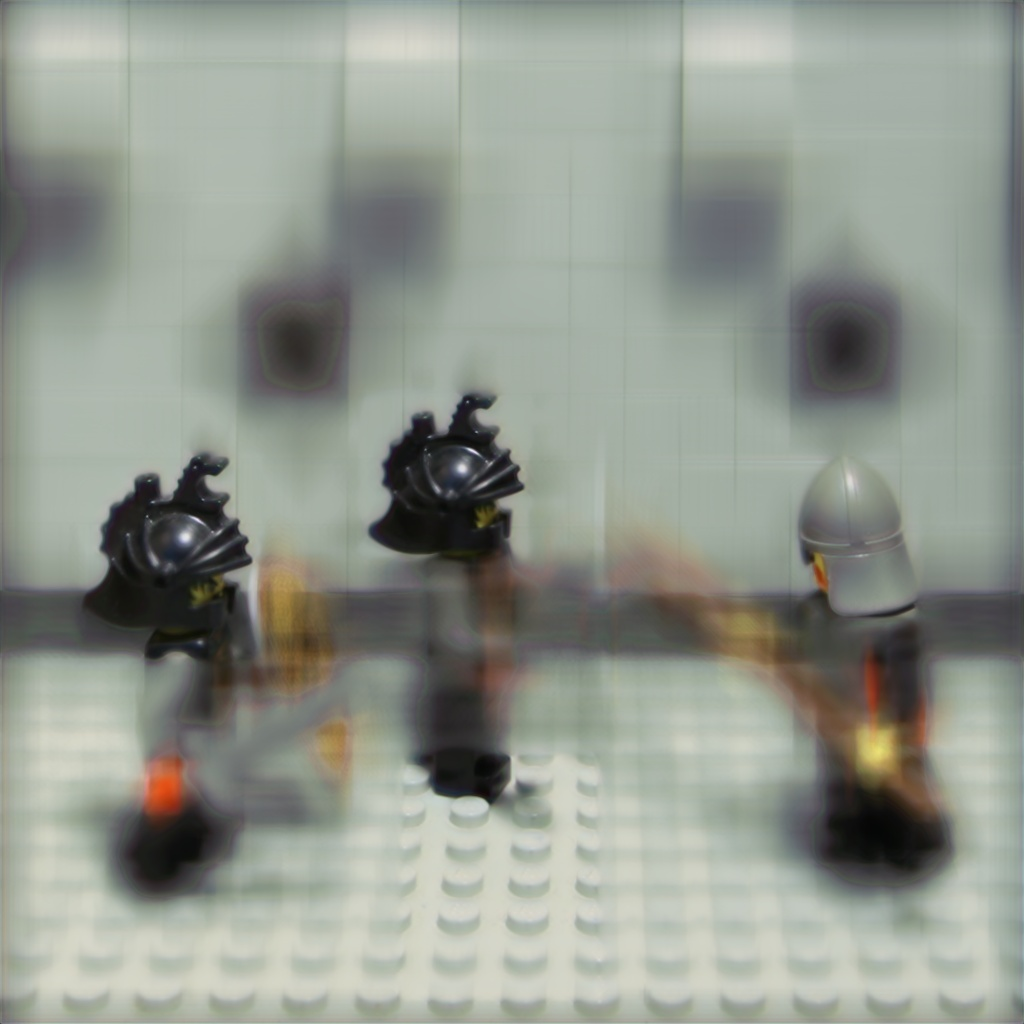}
        %  \caption{ Basler daA1920-30uc (S-Mount)}
        %  \label{fig:three sin x}
     \end{subfigure}
     
    %  \vspace{0.5cm}

% \end{figure*}
% \begin{figure*}[]\ContinuedFloat
     
    \begin{subfigure}[t]{0.29\textwidth}
         \centering
         \includegraphics[width=\textwidth]{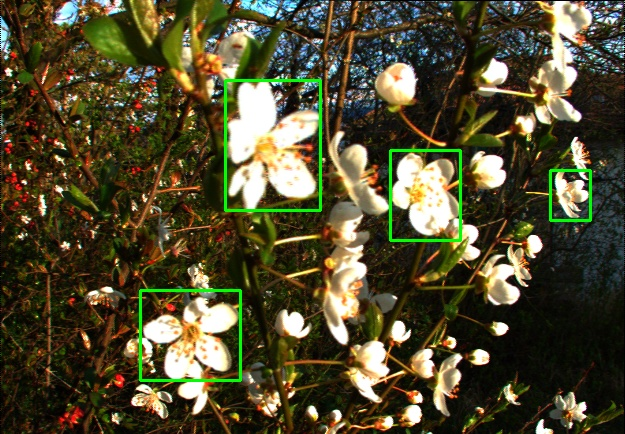}
        %  \caption{\small Evetar Lens M13B0618W}
        %  \label{fig:y equals x}
     \end{subfigure}
     \hspace{0.1cm}
    \begin{subfigure}[t]{0.29\textwidth}
         \centering
         \includegraphics[width=\textwidth]{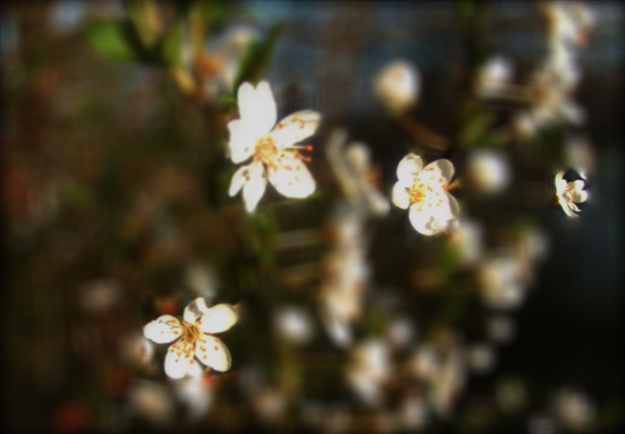}
         \caption{}
        %  \label{fig:y equals x}
     \end{subfigure}
     \hspace{0.1cm}
     \begin{subfigure}[t]{0.29\textwidth}
         \centering
         \includegraphics[width=\textwidth]{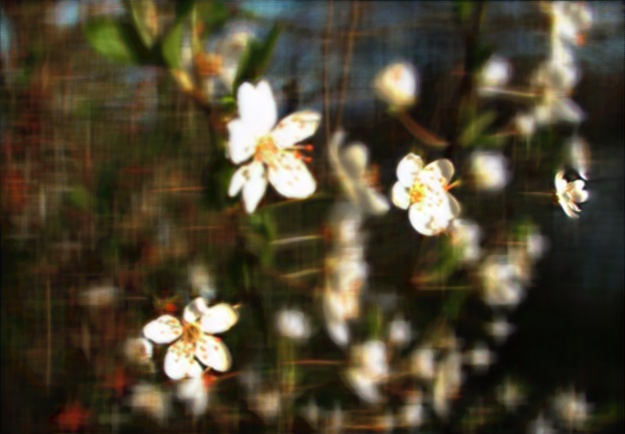}
        %  \caption{ Basler daA1920-30uc (S-Mount)}
        %  \label{fig:three sin x}
     \end{subfigure}

    \begin{subfigure}[t]{0.29\textwidth}
         \centering
         \includegraphics[width=\textwidth]{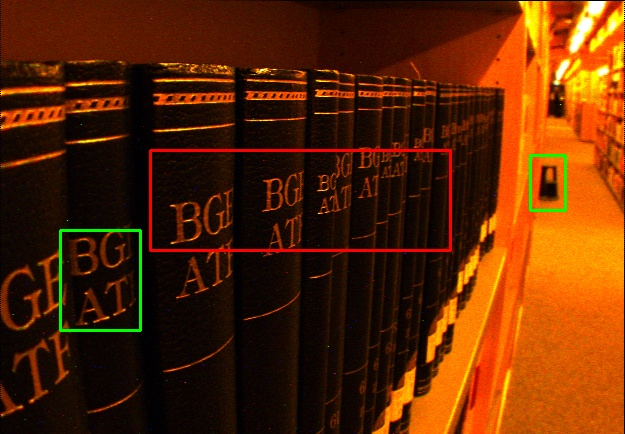}
        %  \caption{\small Evetar Lens M13B0618W}
        %  \label{fig:y equals x}
     \end{subfigure}
     \hspace{0.1cm}
    \begin{subfigure}[t]{0.29\textwidth}
         \centering
         \includegraphics[width=\textwidth]{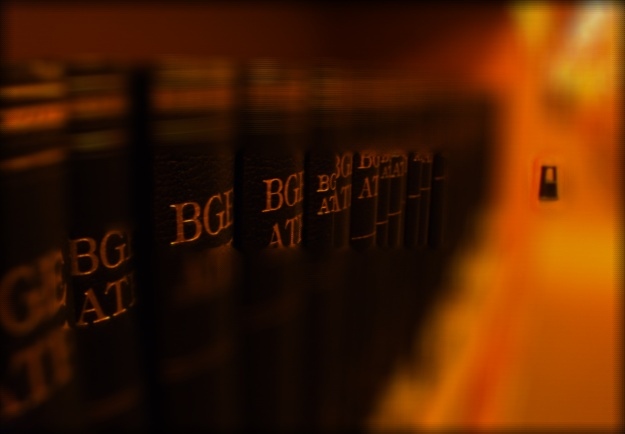}
         \caption{}
        %  \label{fig:y equals x}
     \end{subfigure}
     \hspace{0.1cm}
     \begin{subfigure}[t]{0.29\textwidth}
         \centering
         \includegraphics[width=\textwidth]{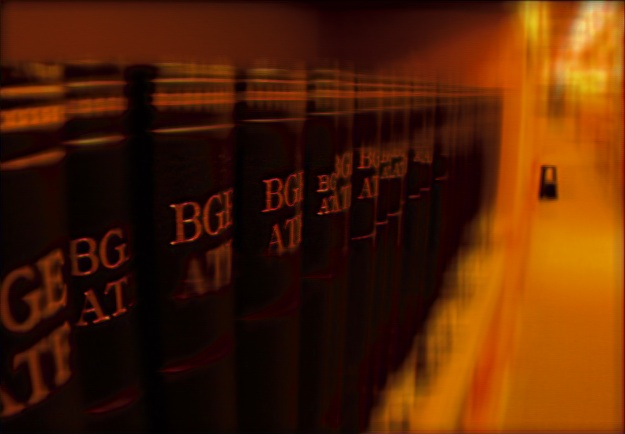}
        %  \caption{ Basler daA1920-30uc (S-Mount)}
        %  \label{fig:three sin x}
     \end{subfigure}
     
    %  \vspace{0.5cm}
     
    \begin{subfigure}[t]{0.29\textwidth}
         \centering
         \includegraphics[width=\textwidth]{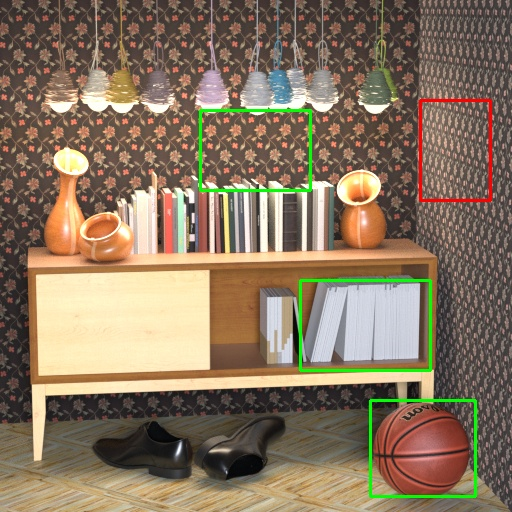}
        %  \caption{\small Evetar Lens M13B0618W}
        %  \label{fig:y equals x}
     \end{subfigure}
     \hspace{0.1cm}
    \begin{subfigure}[t]{0.29\textwidth}
         \centering
         \includegraphics[width=\textwidth]{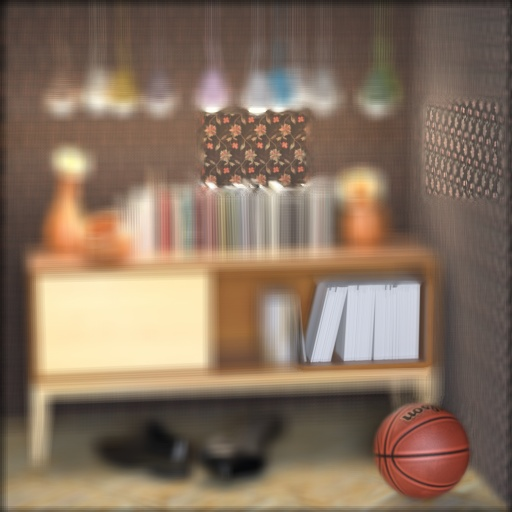}
         \caption{}
        %  \label{fig:y equals x}
     \end{subfigure}
     \hspace{0.1cm}
     \begin{subfigure}[t]{0.29\textwidth}
         \centering
         \includegraphics[width=\textwidth]{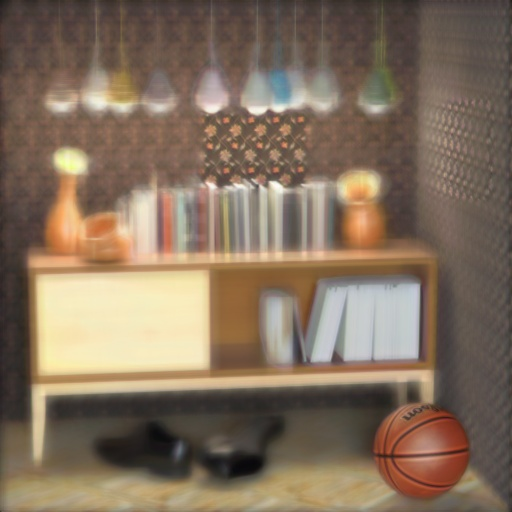}
        %  \caption{ Basler daA1920-30uc (S-Mount)}
        %  \label{fig:three sin x}
     \end{subfigure}

    \caption{Multi arbitrary-volume refocusing qualitative results. (a) Lego Knights LF from Stanford LF dataset~\cite{stanfordnewdataset}, (b) Mirabelle Prune Tree, (c) Books LFs from EPFL LF dataset~\cite{epfldataset}, (d) Sideboard LF from HCI LF dataset~\cite{hcidataset}. ROIs in green color boxes $\in \mathfrak{R}_{s}$ and ROIs in red color boxes $\in \mathfrak{R}_{w}$.}
    \label{fig:qualitative}
\end{figure*}
